# Supplementary material for: Learning to Read Analog Gauges from Synthetic Data
Source: arXiv:2308.14583 source file (2023-08-28)
Supplement: Supplementary file 1 [file Appendix.tex]

\label{sec:appendix}
